# Supplementary material for: Measurement of the $W$-boson mass in pp collisions at $\sqrt{s}=7$ TeV with the ATLAS detector
Source: arXiv:1701.07240 source file (2018-11-07)
Supplement: Supplementary file 1 [file Appendix.tex]

\clearpage
\newpage
\appendix

\section{Appendix}
\label{App:crosssection}

We foresee to present here all additional tables of the measured cross-sections.

\input{figures/SamuelWebb/lowmass_y0008_paper.tex}
\input{figures/SamuelWebb/lowmass_y0816_paper.tex}
\input{figures/SamuelWebb/lowmass_y1624_paper.tex}
\input{figures/SamuelWebb/lowmass_allrapidity_paper.tex}

\input{figures/SamuelWebb/peakmass_y0004_paper.tex}
\input{figures/SamuelWebb/peakmass_y0408_paper.tex}
\input{figures/SamuelWebb/peakmass_y0812_paper.tex}
\input{figures/SamuelWebb/peakmass_y1216_paper.tex}
\input{figures/SamuelWebb/peakmass_y1620_paper.tex}
\input{figures/SamuelWebb/peakmass_y2024_paper.tex}
\input{figures/SamuelWebb/peakmass_allrapidity_paper.tex}

\input{figures/SamuelWebb/highmass_y0008_paper.tex}
\input{figures/SamuelWebb/highmass_y0816_paper.tex}
\input{figures/SamuelWebb/highmass_allrapidity_paper.tex}

\clearpage 

\input{tables/ZPtM1U2Val.tex}
\input{tables/ZPtVal.tex}
\input{tables/ZPtM3U2Val.tex}
\input{tables/ZPtLowM1Val.tex}
\input{tables/ZPtLowM2Val.tex}
\input{tables/ZPtLowM3Val.tex}

\input{tables/ZPtY1U2Val.tex}
\input{tables/ZPtY2U2Val.tex}
\input{tables/ZPtY3U2Val.tex}
\input{tables/ZPtY4U2Val.tex}
\input{tables/ZPtY5U2Val.tex}
\input{tables/ZPtY6U2Val.tex}
